# Supplementary material for: Think Before Refusal : Triggering Safety Reflection in LLMs to Mitigate False Refusal Behavior
Source: arXiv:2503.17882 source file (2025-03-22)
Supplement: Supplementary file 1 [file result_appendix.tex]

\begin{table*}[t]
    \centering
    \small
    \begin{tabular}[!t]{l cc cc ccc} % 根据需要调整列数和对齐方式
        \toprule
        \multirow{3}{*}{} & \multicolumn{2}{c}{\textbf{Safety}} & \multicolumn{2}{c}{\textbf{Oversensitivity}} & \multicolumn{3}{c}{\textbf{General Performance}} \\
        \cmidrule[0.3pt](lr){2-3} \cmidrule(lr){4-5} \cmidrule(lr){6-8}
           & \textbf{Xstest-H} &\textbf{Malicious} & \textbf{Xstest-S} & \textbf{OR-Bench} & \textbf{MLLU} & \textbf{GSM8K} & \textbf{ARC-E} \\
           & CR $\downarrow$ & CR $\downarrow$ & CR $\uparrow$ & CR $\uparrow$  & CR $\uparrow$  & CR $\uparrow$ & CR $\uparrow$  \\
        \midrule
        \gemmaonetwob \\
        \hspace{10pt} Fine-Tuned w/o Rationale & 0.10 & 0.07 & 0.74 & 0.68 & 0.31 & 0.12 & 0.71\\
        \hspace{10pt} Fine-Tuned w/ \ \  Internal Rationale & 0.13 & 0.12 & 0.78 & 0.74 & 0.32 & 0.12 & 0.71 \\
        \hspace{10pt} Fine-Tuned w/ \ \  External Rationale & 0.12 & 0.07 & \textbf{0.79} & \textbf{0.83} & 0.31 & 0.12 & 0.71 \\
        \midrule
        % \gemmaonesevenb \\
        % \hspace{10pt} Fine-Tuned w/o Rationale & 0.02 & 0.04 & 0.71 & 0.64 & 0.53 & 0.44 & 0.81\\
        % \hspace{10pt} Fine-Tuned w/ \ \  Internal Rationale & 0.05 & 0.01 & 0.82 & 0.71 & 0.51 & 0.42 & 0.81 \\
        % \hspace{10pt} Fine-Tuned w/ \ \  External Rationale & 0.02 & 0.02 & \textbf{0.90} & \textbf{0.75} & 0.54 & 0.42 & 0.79 \\
        % \midrule
        \gemmatwotwob \\
        \hspace{10pt} Fine-Tuned w/o Rationale & 0.17 & 0.16 & 0.89 & 0.71 & 0.45 & 0.21 & 0.78\\
        \hspace{10pt} Fine-Tuned w/ \ \  Internal Rationale & 0.20 & 0.20 & 0.90 & 0.80 & 0.46 & 0.21 & 0.79 \\
        \hspace{10pt} Fine-Tuned w/ \ \  External Rationale & 0.20 & 0.11 & \textbf{0.91} & \textbf{0.73} & 0.46 & 0.20 & 0.78 \\
        \midrule
        \gemmatwonineb \\
        \hspace{10pt} Fine-Tuned w/o Rationale & 0.04 & 0.07 & 0.85 & 0.64 & 0.66 & 0.60 & 0.85\\
        \hspace{10pt} Fine-Tuned w/ \ \  Internal Rationale & 0.07 & 0.10 & 0.88 & 0.68 & 0.66 & 0.61 & 0.86 \\
        \hspace{10pt} Fine-Tuned w/ \ \  External Rationale & 0.05 & 0.03 & \textbf{0.90} & \textbf{0.72} & 0.67 & 0.60 & 0.86 \\
        \midrule
        % \llamaonesevenb \\
        % \hspace{10pt} Fine-Tuned w/o Rationale & 0.01 & 0.01 & 0.69 & 0.48 & 0.33 & 0.09 & 0.75\\
        % \hspace{10pt} Fine-Tuned w/ \ \  Internal Rationale & 0.02 & 0.05 & 0.89 & 0.54 & 0.33 & 0.10 & 0.75 \\
        % \hspace{10pt} Fine-Tuned w/ \ \  External Rationale & 0.02 & 0.01 & \textbf{0.91} & \textbf{0.62} & 0.32 & 0.10 & 0.75 \\
        % \midrule
        % \llamatwosevenb \\
        % \hspace{10pt} Fine-Tuned w/o Rationale & 0.02 & 0.03 & 0.74 & 0.74 & 0.41 & 0.13 & 0.76 \\
        % \hspace{10pt} Fine-Tuned w/ \ \  Internal Rationale & 0.03 & 0.05 & 0.79 & 0.75 & 0.40 & 0.13 & 0.75 \\
        % \hspace{10pt} Fine-Tuned w/ \ \  External Rationale & 0.03 & 0.04 & \textbf{0.92} & \textbf{0.80} & 0.42 & 0.13 & 0.76 \\
        % \midrule
        \llamaonethirteenb \\
        \hspace{10pt} Fine-Tuned w/o Rationale & 0.00 & 0.00 & 0.66 & 0.26 & 0.42 & 0.16 & 0.77\\
        \hspace{10pt} Fine-Tuned w/ \ \  Internal Rationale & 0.02 & 0.03 & 0.80 & 0.37 & 0.41 & 0.16 & 0.77 \\
        \hspace{10pt} Fine-Tuned w/ \ \  External Rationale & 0.01 & 0.01 & \textbf{0.89} & \textbf{0.41} & 0.43 & 0.16 & 0.77  \\
        \bottomrule
    \end{tabular}
    \caption{Compliance Rate (CR) on safety and oversensitivity datasets, and Accuracy (ACC) on general performance benchmarks were evaluated. With safety-reflection fine-tuning, the compliance rate on oversensitivity datasets improves across all models, while safety and general performance remain largely unchanged. }
    \label{table:appendix}
\end{table*}
